# Supplementary material for: Matching Anonymized and Obfuscated Time Series to Users' Profiles
Source: arXiv:1710.00197 source file (2018-06-28)
Supplement: Supplementary file 3 [file appendix_c.tex]

\section{Proof of Lemma \ref{lemOnePointFive}}
\label{sec:app_b}
Here we provide a formal proof for Lemma \ref{lemOnePointFive} which we restate as follows.

Let $N$ be a positive integer, and let $a_1, a_2, \cdots, a_N$ and $b_1, b_2, \cdots, b_N$ be real numbers such that $a_u \leq b_u$ for all $u$. Assume that $X_1, X_2, \cdots, X_N$ are $N$ independent random variables such that
\[X_u \sim Uniform[a_u,b_u]. \]
Let also $\gamma_1, \gamma_2, \cdots, \gamma_N$ be real numbers such that
\[ \gamma_j \in \bigcap_{u=1}^{N} [a_u, b_u] \ \ \textrm{for all }j \in \{1,2,\cdots,N\}. \]
Suppose that we know the event $E$ has occurred, meaning that the observed values of $X_u$'s is equal to the set of $\gamma_j$'s (but with unknown ordering), i.e.,
\[E \ \ \equiv \ \ \{X_1,X_2,\cdots,X_N\}= \{ \gamma_1, \gamma_2, \cdots, \gamma_N \}, \] then
\[P\left(X_1=\gamma_j |E\right)=\frac{1}{N}. \]

\begin{proof}
Define sets $\mathfrak{P}$ and $\mathfrak{P}_j$ as follows:
\[\mathfrak{P}= \textrm{The set of all permutations $\Pi$ on }\{1,2,\cdots,N\}. \]
\[\mathfrak{P}_j= \textrm{The set of all permutations $\Pi$ on }\{1,2,\cdots,N\} \textrm{ such that } \Pi(1)=j. \]
We have $|\mathfrak{P}|=N!$ and $|\mathfrak{P}|=(N-1)!$. Then
\begin{align*}
 P(X_1=\alpha_j |E)&=\frac{\sum_{\pi \in \mathfrak{P}_j} f_{X_1,X_2, \cdots,X_N} (\gamma_{\pi(1)}, \gamma_{\pi(2)}, \cdots, \gamma_{\pi(N)})} {\sum_{\pi \in \mathfrak{P}} f_{X_1,X_2, \cdots,X_N} (\gamma_{\pi(1)}, \gamma_{\pi(2)}, \cdots, \gamma_{\pi(N)})}\\
 &=\frac{(N-1)! \prod\limits_{u=1}^{N} \frac{1}{b_u-a_u}}{N! \prod\limits_{u=1}^{N} \frac{1}{b_u-a_u}}\\
 &=\frac{1}{N}.
\end{align*}
\end{proof}
